# Supplementary material for: Distribution of interseismic coupling along the North and East Anatolian Faults inferred from InSAR and GPS data
Source: arXiv:2003.02001 source file (2020-07-17)
Supplement: Supplementary file 1 [file revised_supplements_compressed.pdf]

# Supporting Information for "Distribution of interseismic coupling along the North and East Anatolian Faults inferred from InSAR and GPS data"

Quentin Bletery[1], Olivier Cavalié[1], Jean-Mathieu Nocquet[1,2] and Théa Ragon[3]

[1]Université Côte d'Azur, IRD, CNRS, Observatoire de la Côte d'Azur, Géoazur, France

[2]Institut de Physique du Globe de Paris, Université de Paris, CNRS, France

[3]Seismological Laboratory, California Institute of Technology, USA

## Contents of this file

1. Figures S1 to S17

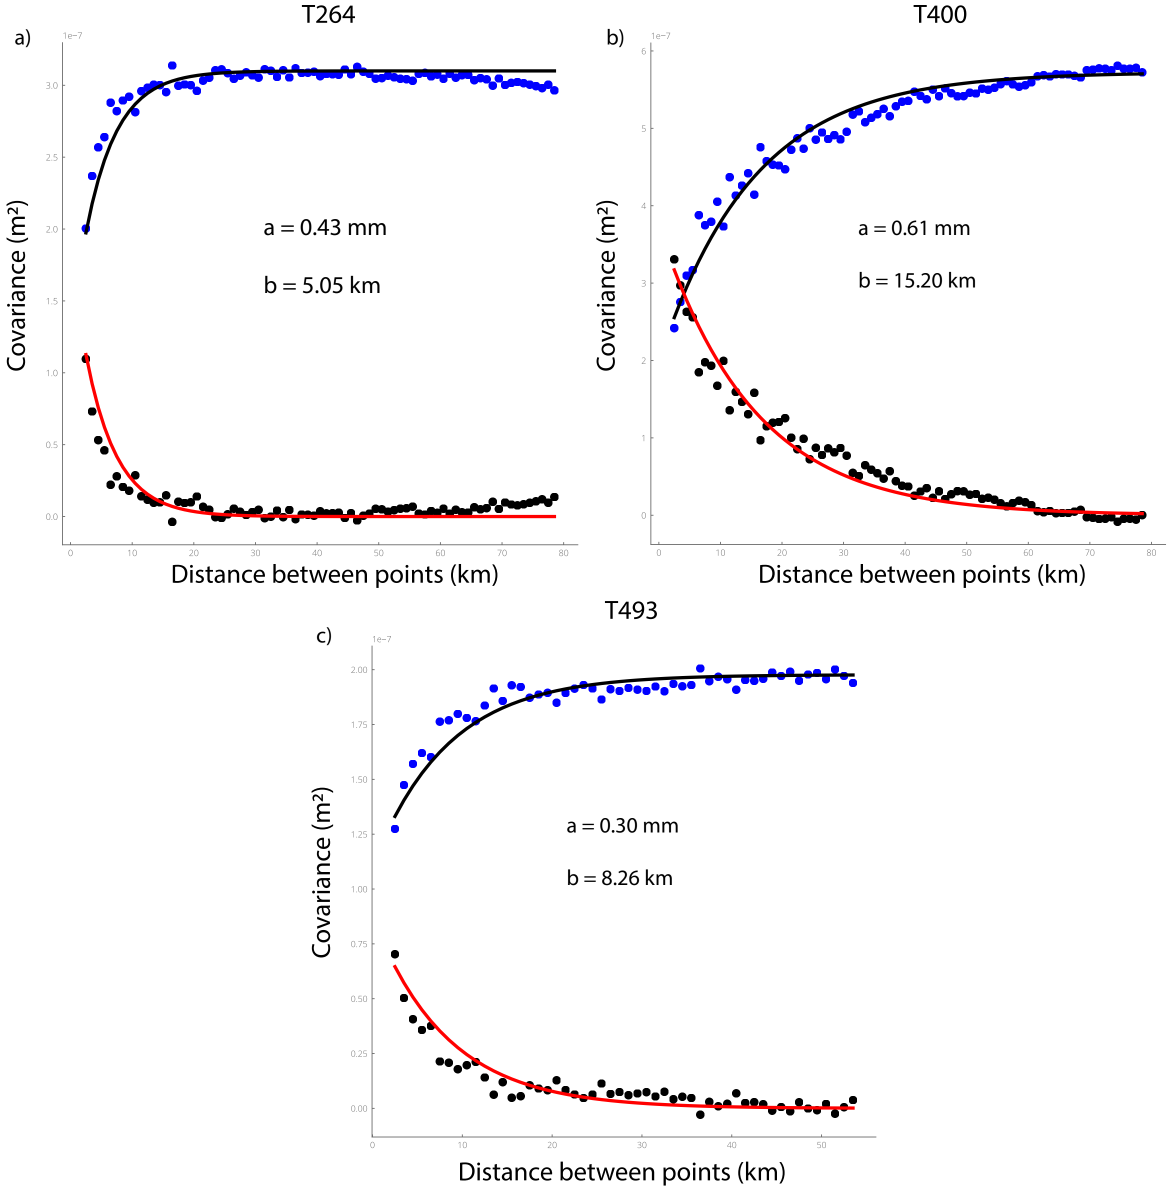


**Figure S1.** Covariance between InSAR pixels as a function of distance and fits of a and b parameters in equation (2).

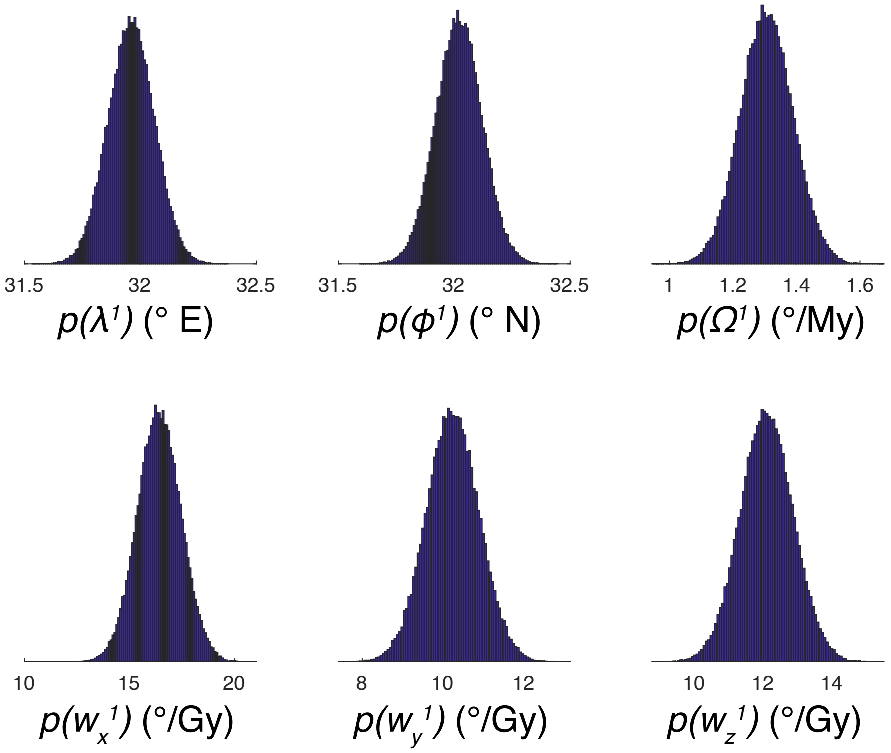


**Figure S2.** Top: prior pdfs of the Euler pole coordinates $p(\lambda^1)$, $p(\phi^1)$ and angular velocity $p(\Omega^1)$ of the Anatolian plate with respect to Eurasia. Bottom: corresponding prior pdfs of the rotation vector in Cartesian geocentric coordinates (in $10^{-9}$ °/y). The obtained means of the distributions of $w_x^1$, $w_y^1$, $w_z^1$ are 16.4, 10.2 and 12.1 $\times 10^{-9}$ °/y respectively, the standard deviations 1.04, 0.65 and 0.77 $\times 10^{-9}$ °/y. Corresponding numbers in geographic coordinates are given in Table 1.

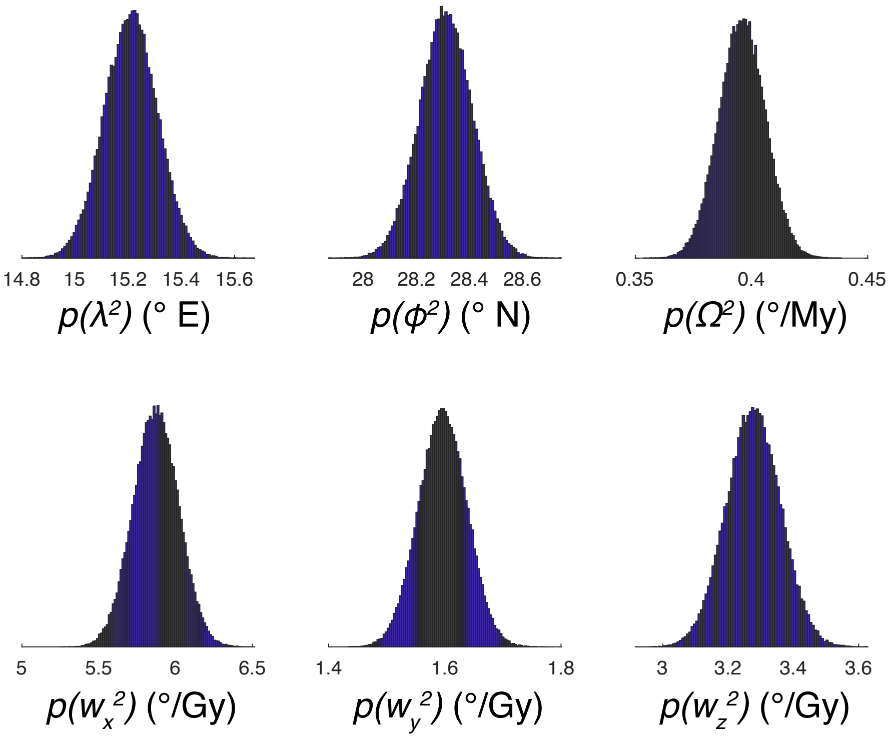


**Figure S3.** Top: prior pdfs of the Euler pole coordinates $p(\lambda^2)$, $p(\phi^2)$ and angular velocity $p(\Omega^2)$ of the Arabian plate with respect to Eurasia. Bottom: corresponding prior pdfs of the rotation vector in Cartesian geocentric coordinates (in $10^{-9}$ °/y). The obtained means of the distributions of $w_x^2$, $w_y^2$, $w_z^2$ are 5.9, 1.6 and 3.3 $\times 10^{-9}$ °/y respectively, the standard deviations 0.15, 0.04 and 0.08 $\times 10^{-9}$ °/y. The corresponding numbers in geographic coordinates are given in Table 1.

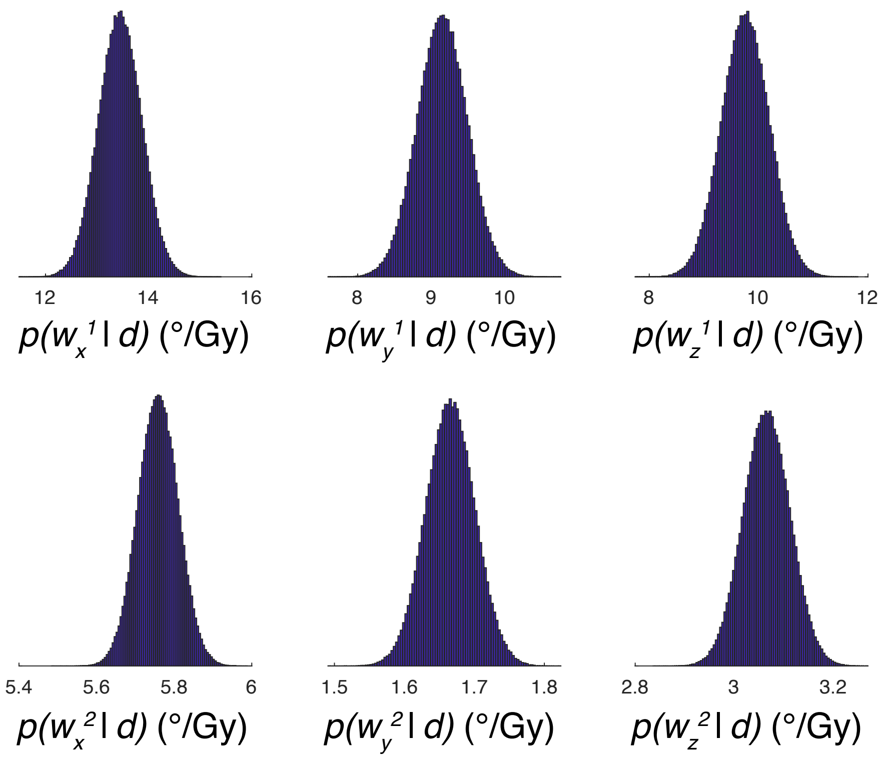


**Figure S4.** Posterior pdfs of the rotation vectors $\mathbf{w^1}$, $\mathbf{w^2}$ in Cartesian geocentric coordinates (in $10^{-9}$ °/y). Means of the posterior pdf distributions of $w_x^1$, $w_y^1$, $w_z^1$ are 13.5, 9.15, 9.76 $\times 10^{-9}$ °/y respectively, standard deviations 0.42, 0.34 and 0.44 $\times 10^{-9}$ °/y. Means of the posterior pdf distributions of $w_x^2$, $w_y^2$, $w_z^2$ are 5.76, 1.67, 3.07 $\times 10^{-9}$ °/y respectively, standard deviations 0.05, 0.04 and 0.05 $\times 10^{-9}$ °/y. Corresponding numbers in geographic coordinates are given in Table 1.

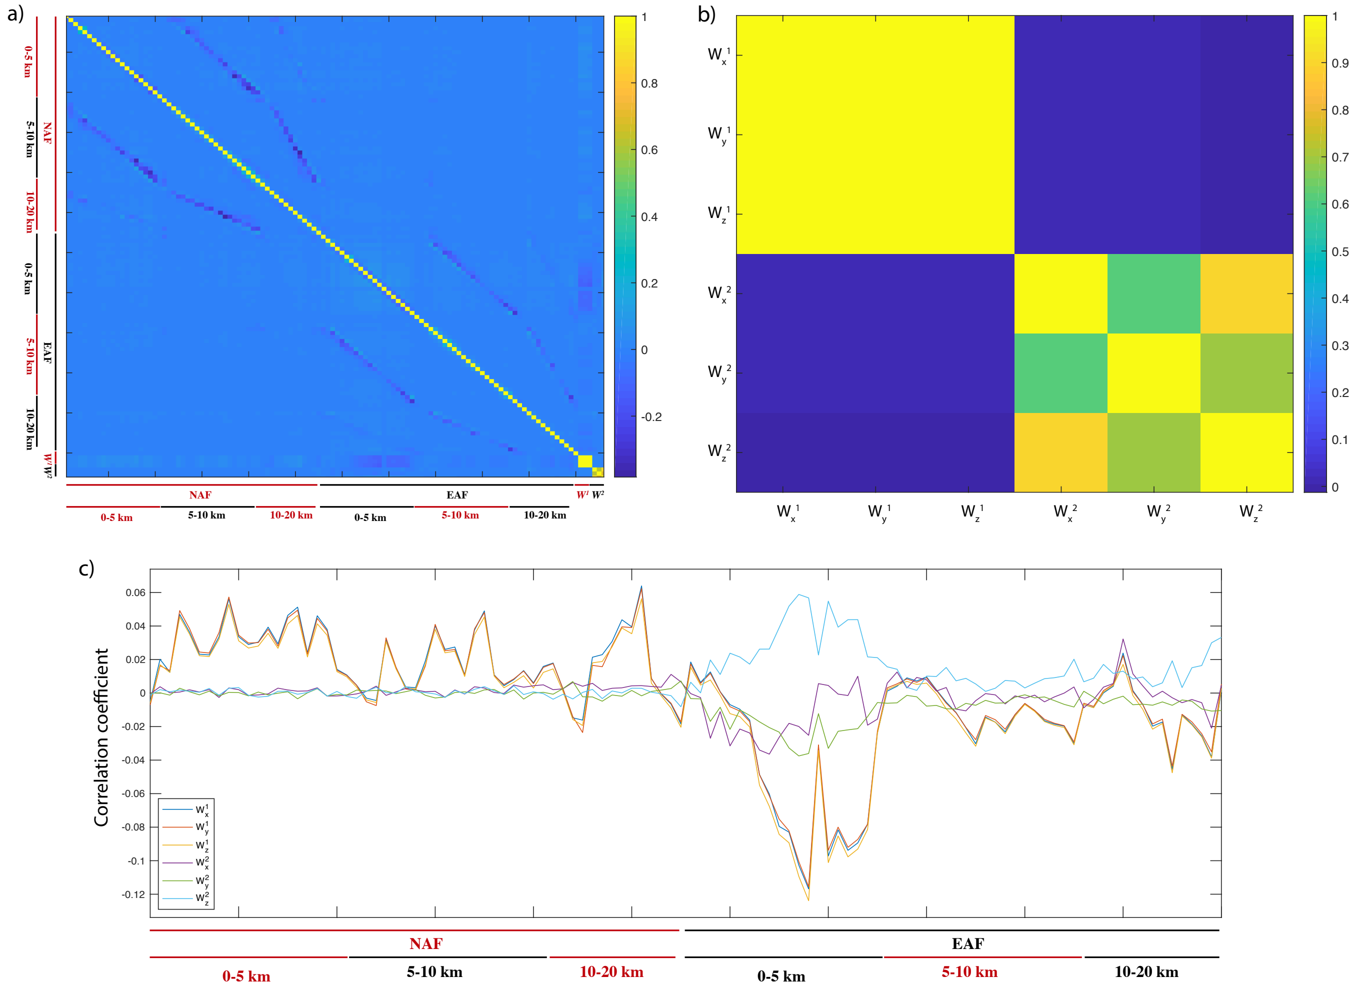


**Figure S5.** Correlations between the posterior pdf distributions of the inverted parameters. a) Correlation matrix of all 116 inverted parameters. The 110 first parameters are fault slip parameters, the last 6 are rotation parameters w. b) Correlation matrix restricted to the 6 w parameters. c) Correlation between each w parameters and all the fault slip parameters. The legend indicates the location of the patches (fault and depth).

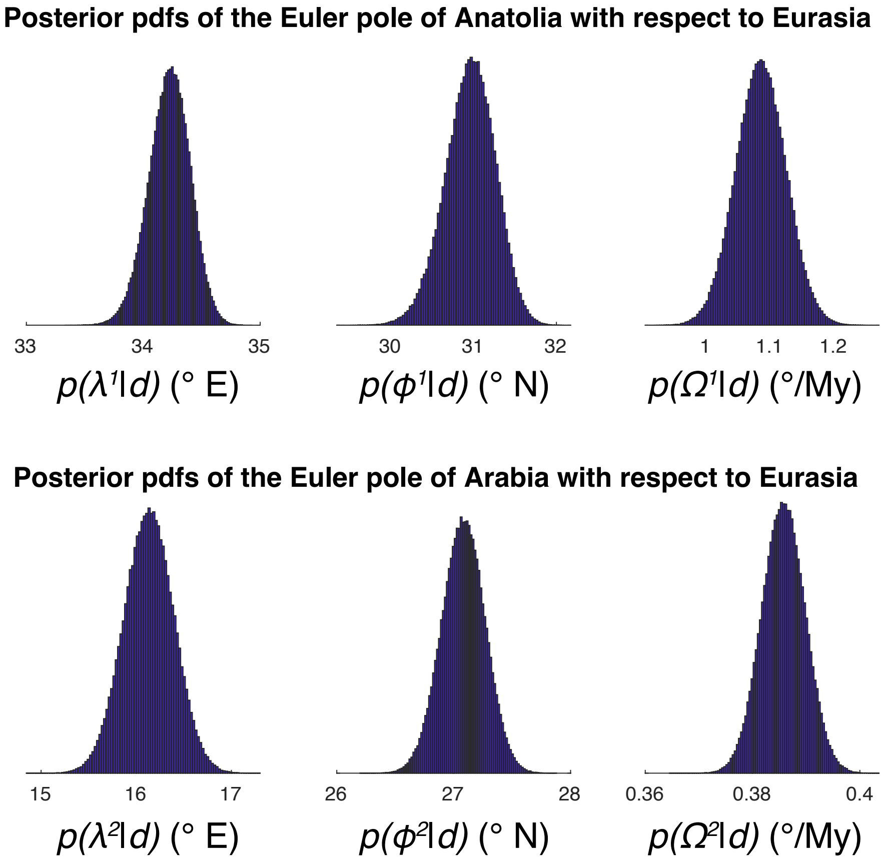


**Figure S6.** Posterior pdfs of the Anatolian and Arabian Euler pole coordinates and angular velocities with respect to Eurasia.

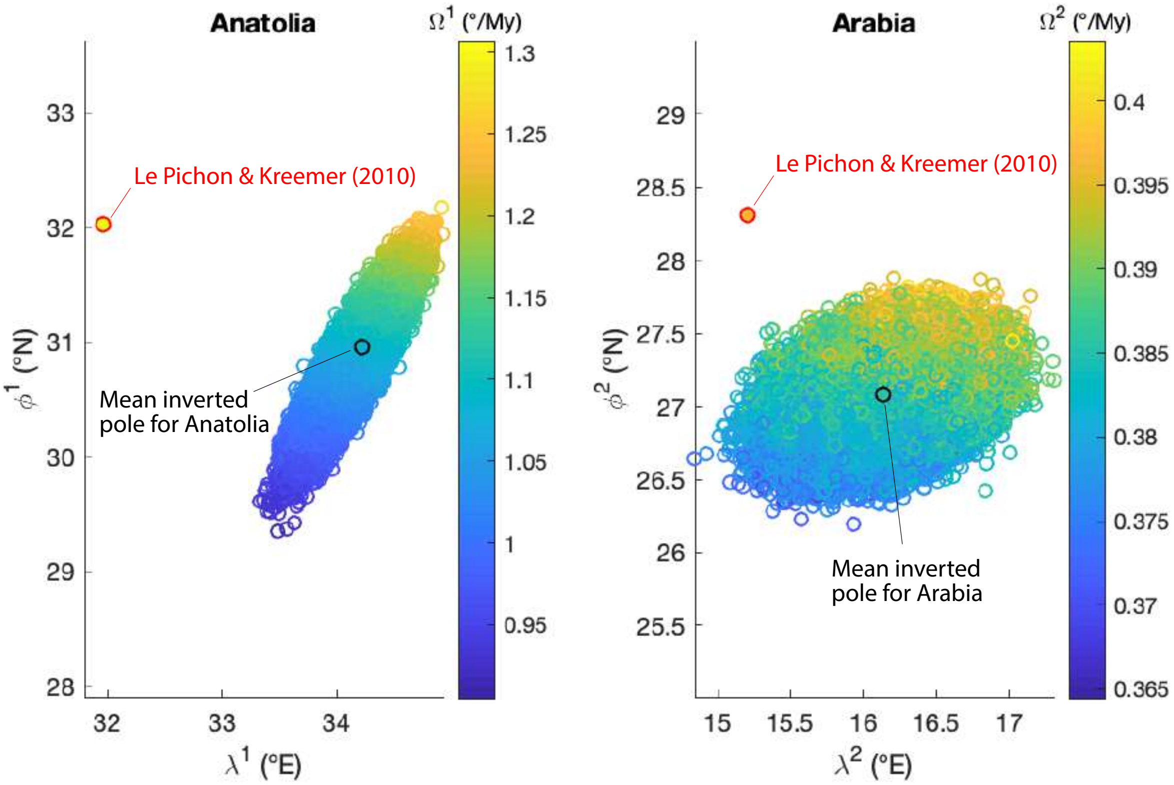


**Figure S7.** Location and angular velocity of all sampled posterior Euler poles in the pdfs of Fig. S6. Red circles show solution from Le Pichon & Kreemer (2010), black circles show the mean of the pdfs.

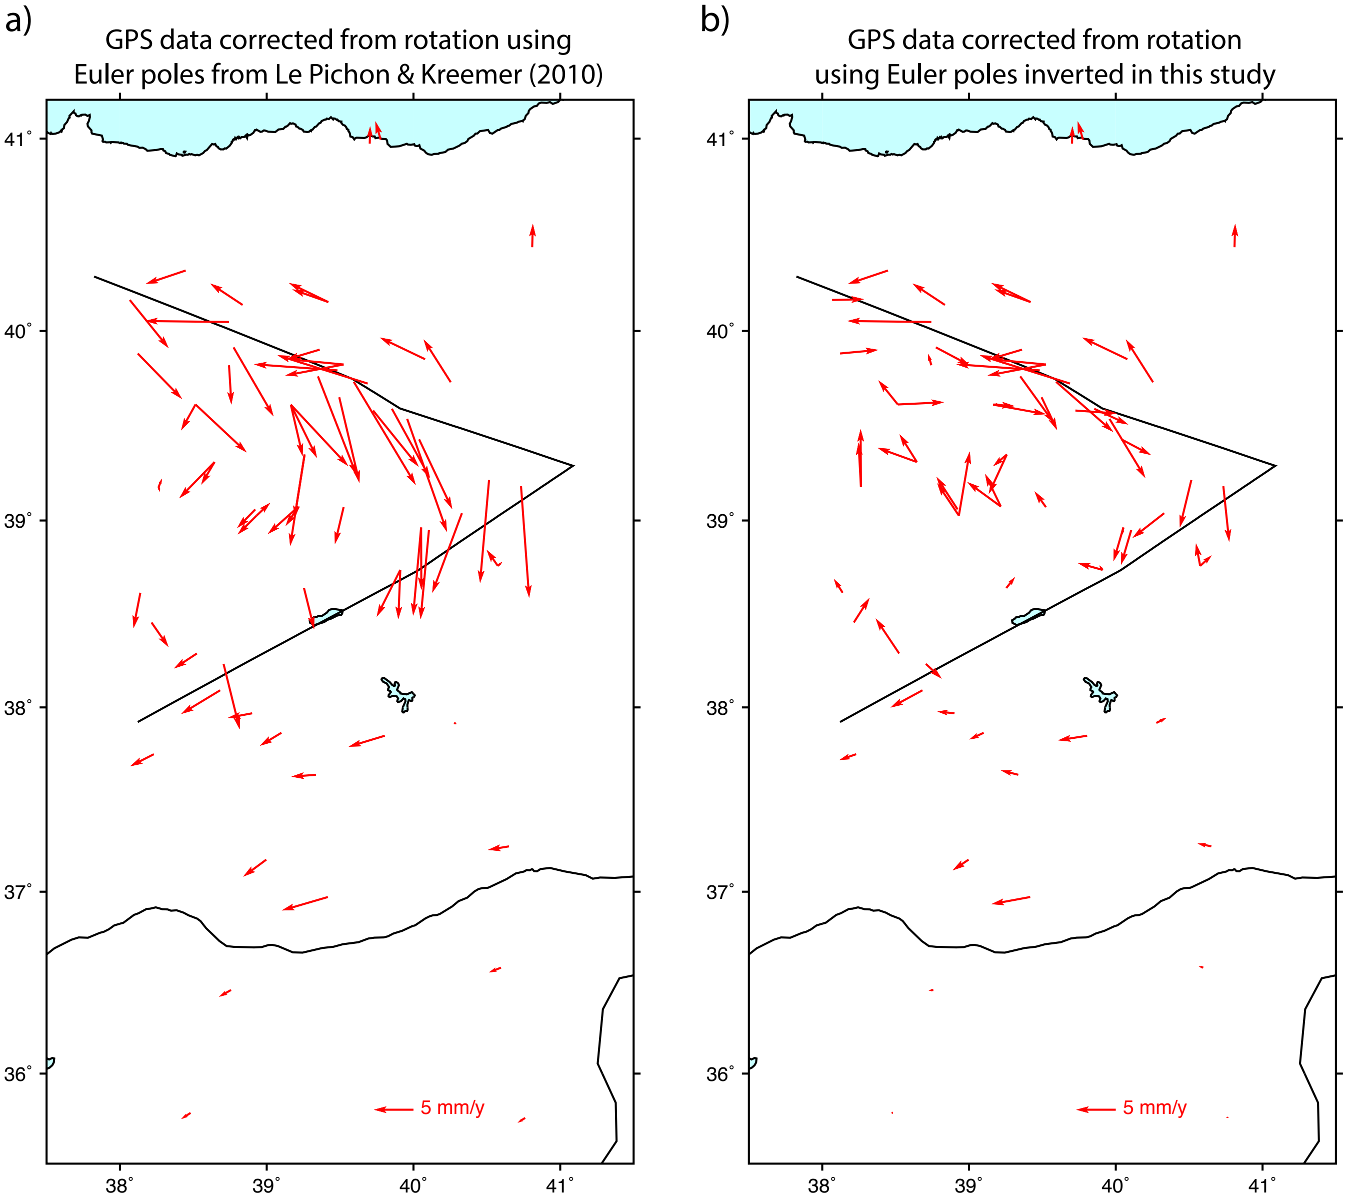


**Figure S8.** GPS data corrected from rotation a) using Euler poles from Le Pichon & Kreemer (2010) and b) using the Euler poles inverted in this study.

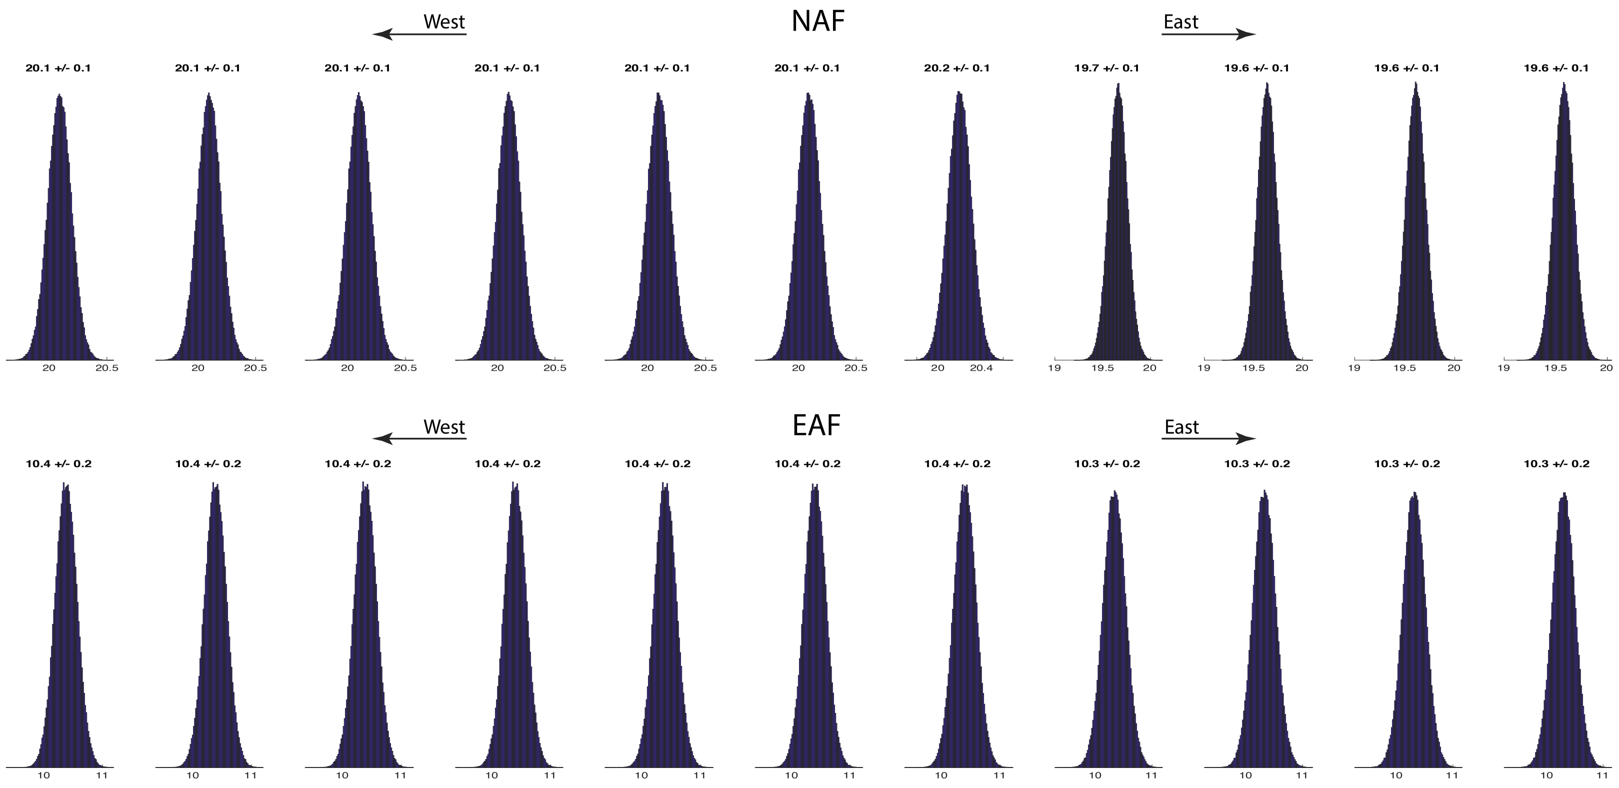


**Figure S9.** Posterior pdfs of long term plate motion rate projected along both faults. Positions correspond to positions of the deepest patches along the faults in Fig. 2. Values at the top of each pdf indicate the pdf mean and standard deviation (in mm/year).

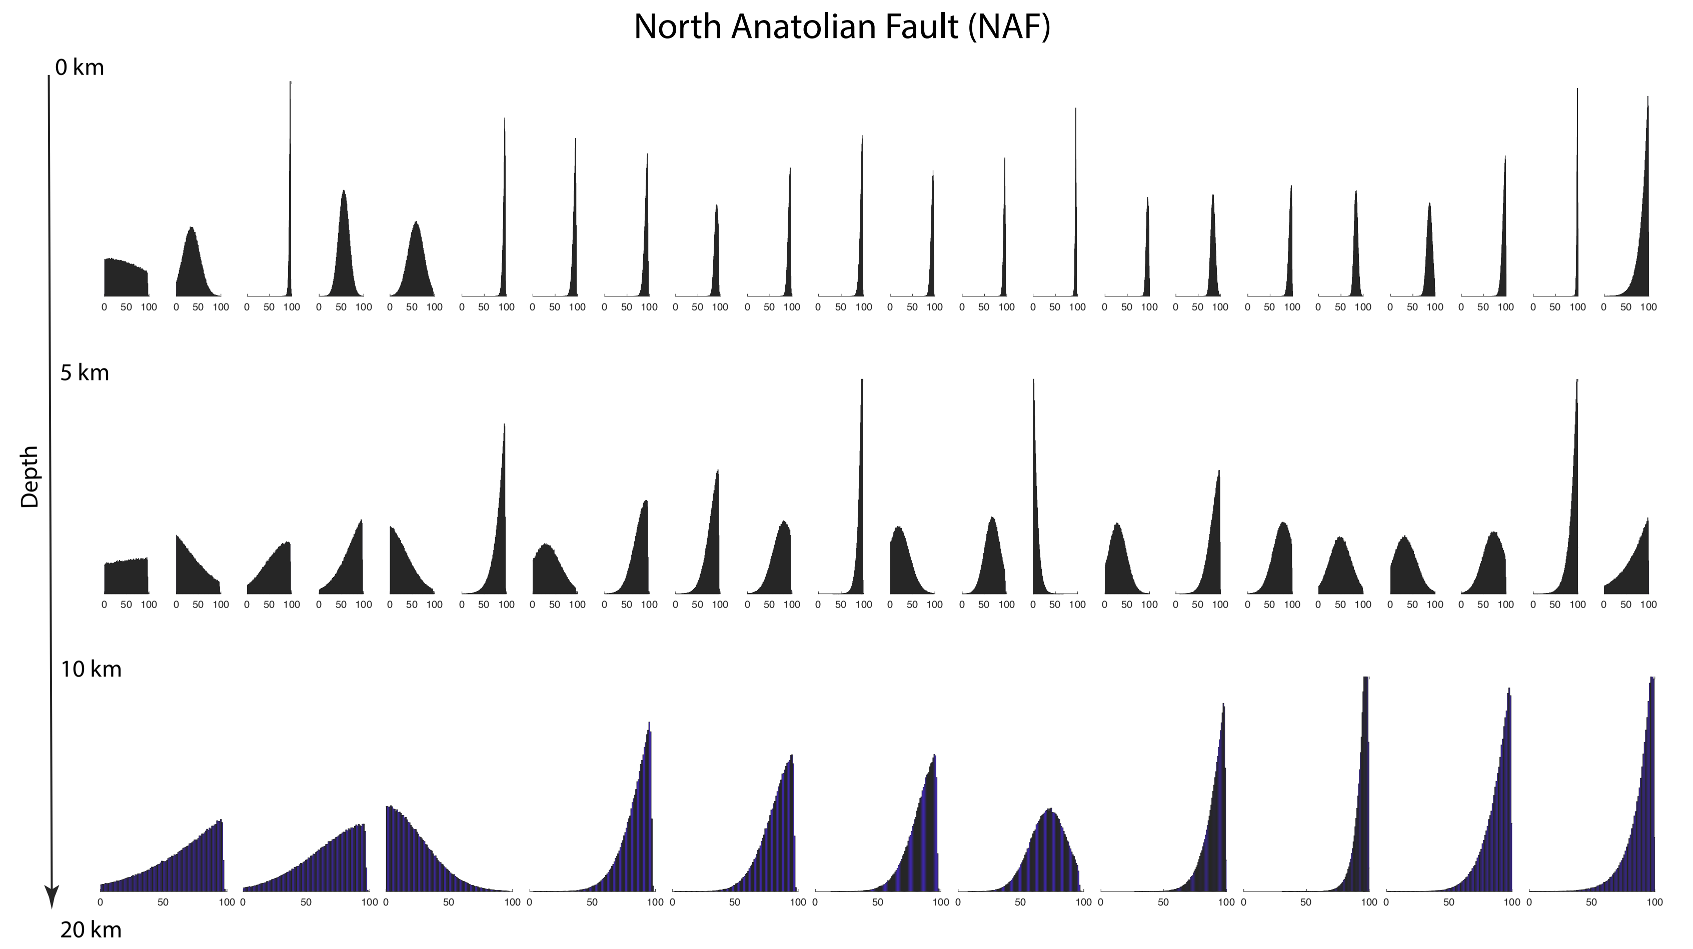


**Figure S10.** Posterior pdfs of each coupling coefficient along the NAF. Positions correspond to positions along the faults in Fig. 2.

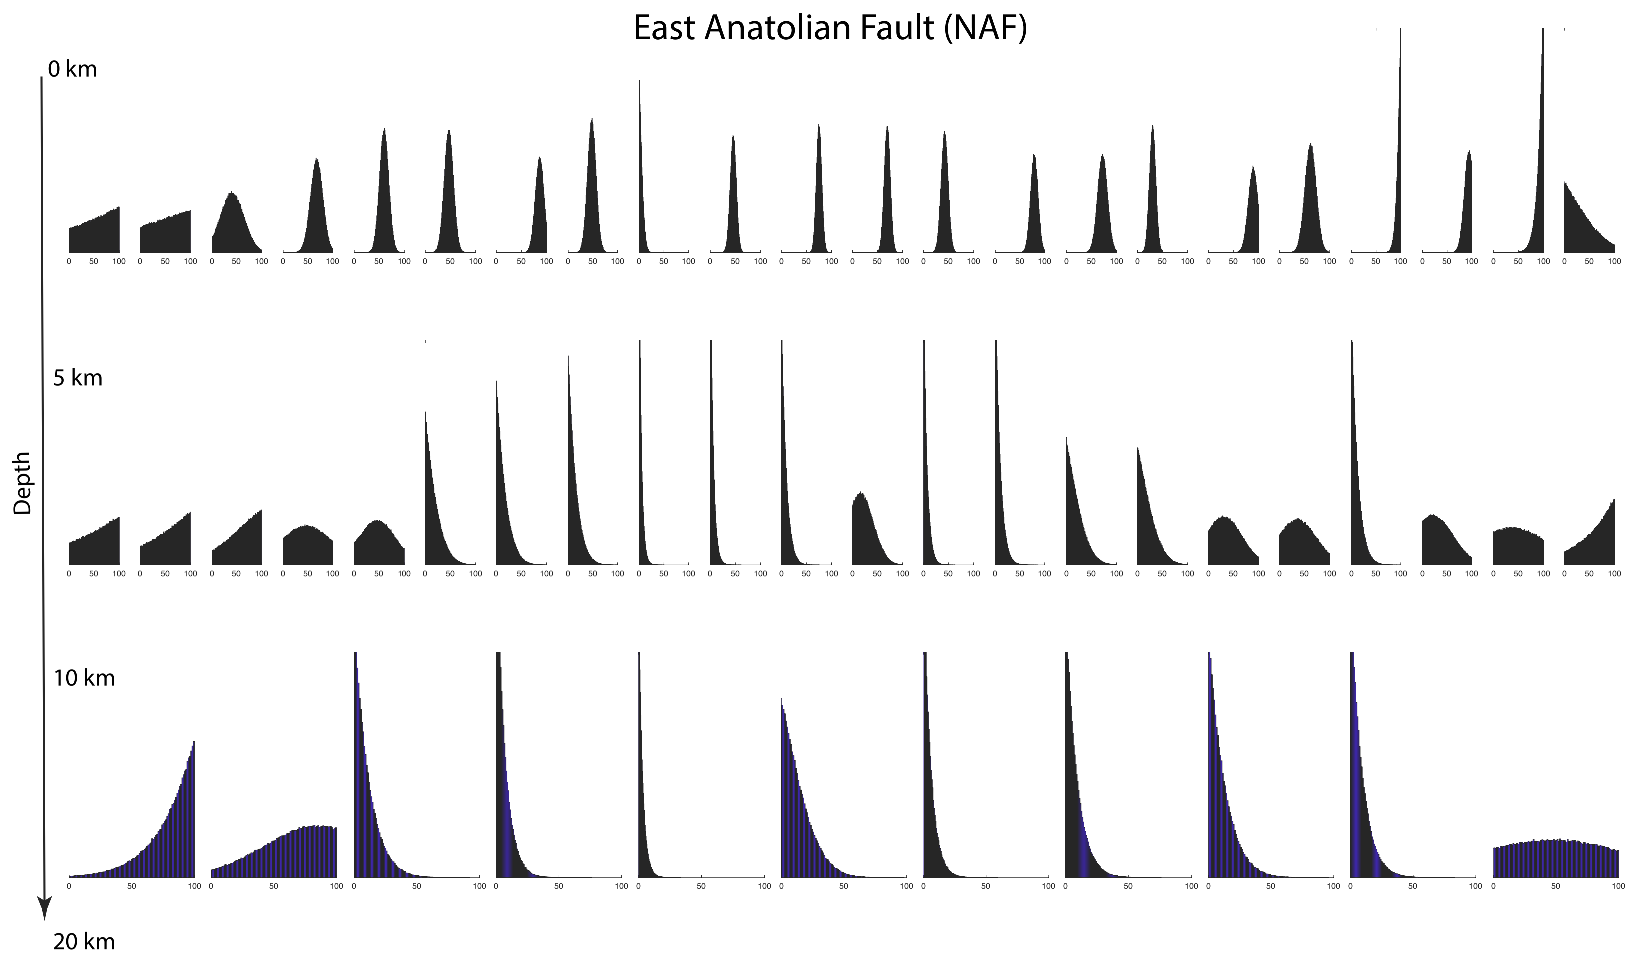


**Figure S11.** Posterior pdfs of each coupling coefficient along the EAF. Positions correspond to positions along the faults in Fig. 2.

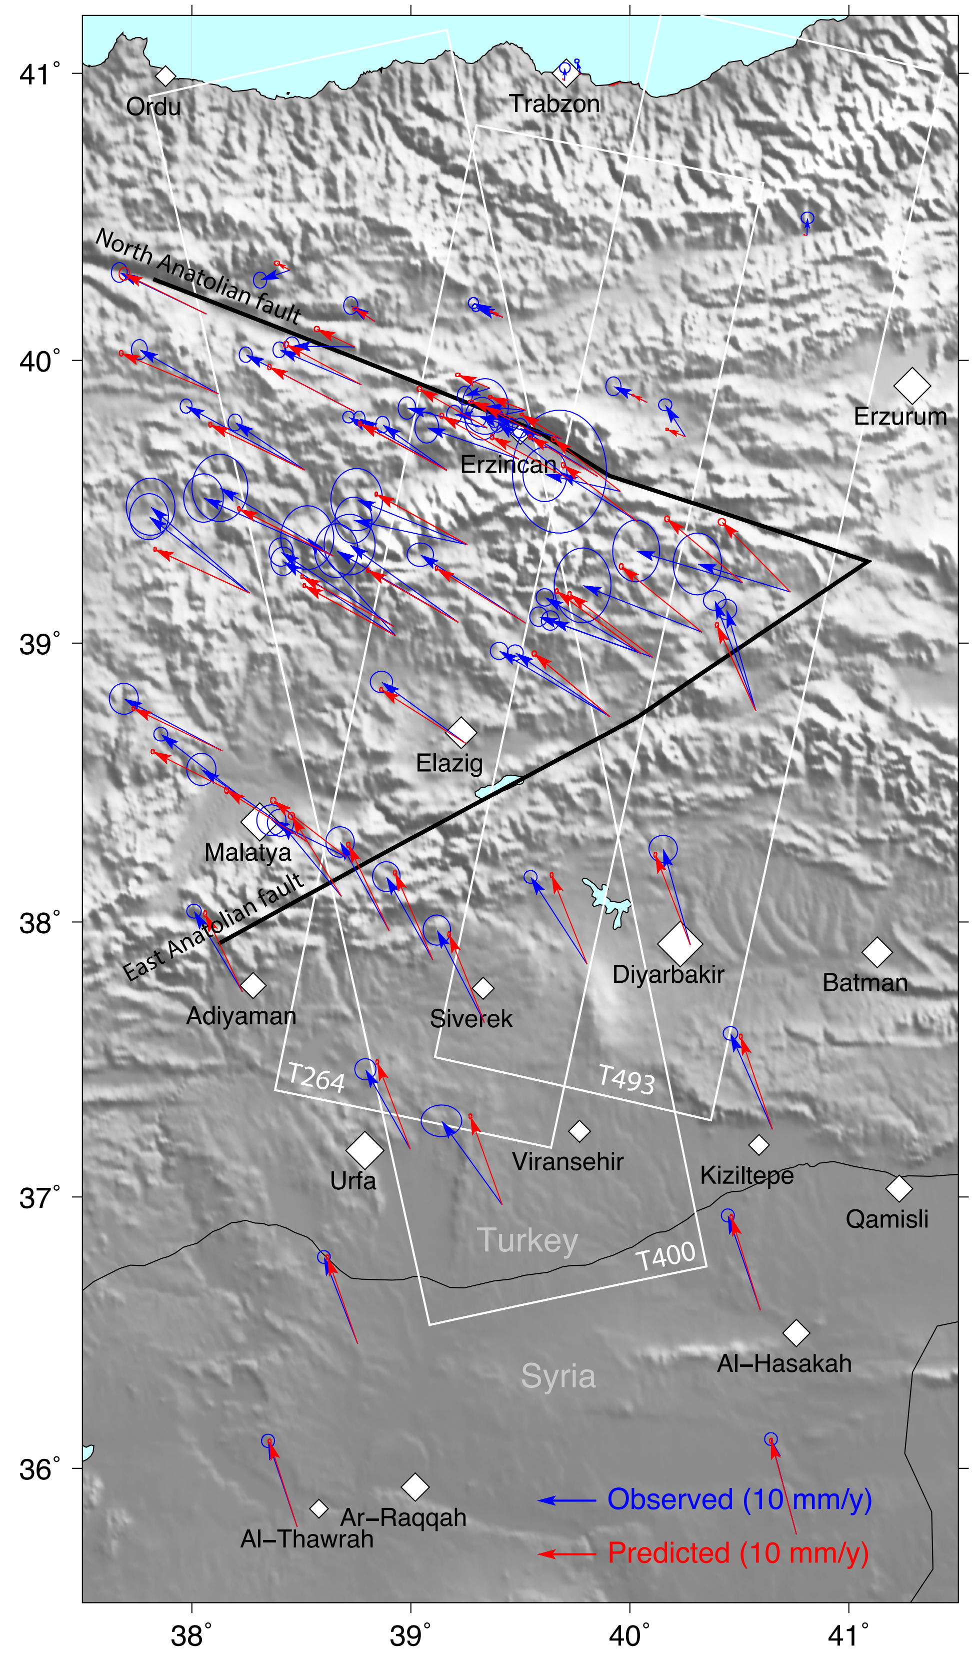


**Figure S12.** Observed (blue) and predicted (red) GPS measurements with their 2-$\sigma$ ellipses of uncertainties. Black lines show the fault traces. White rectangles show the boundaries of the InSAR tracks used in this study.

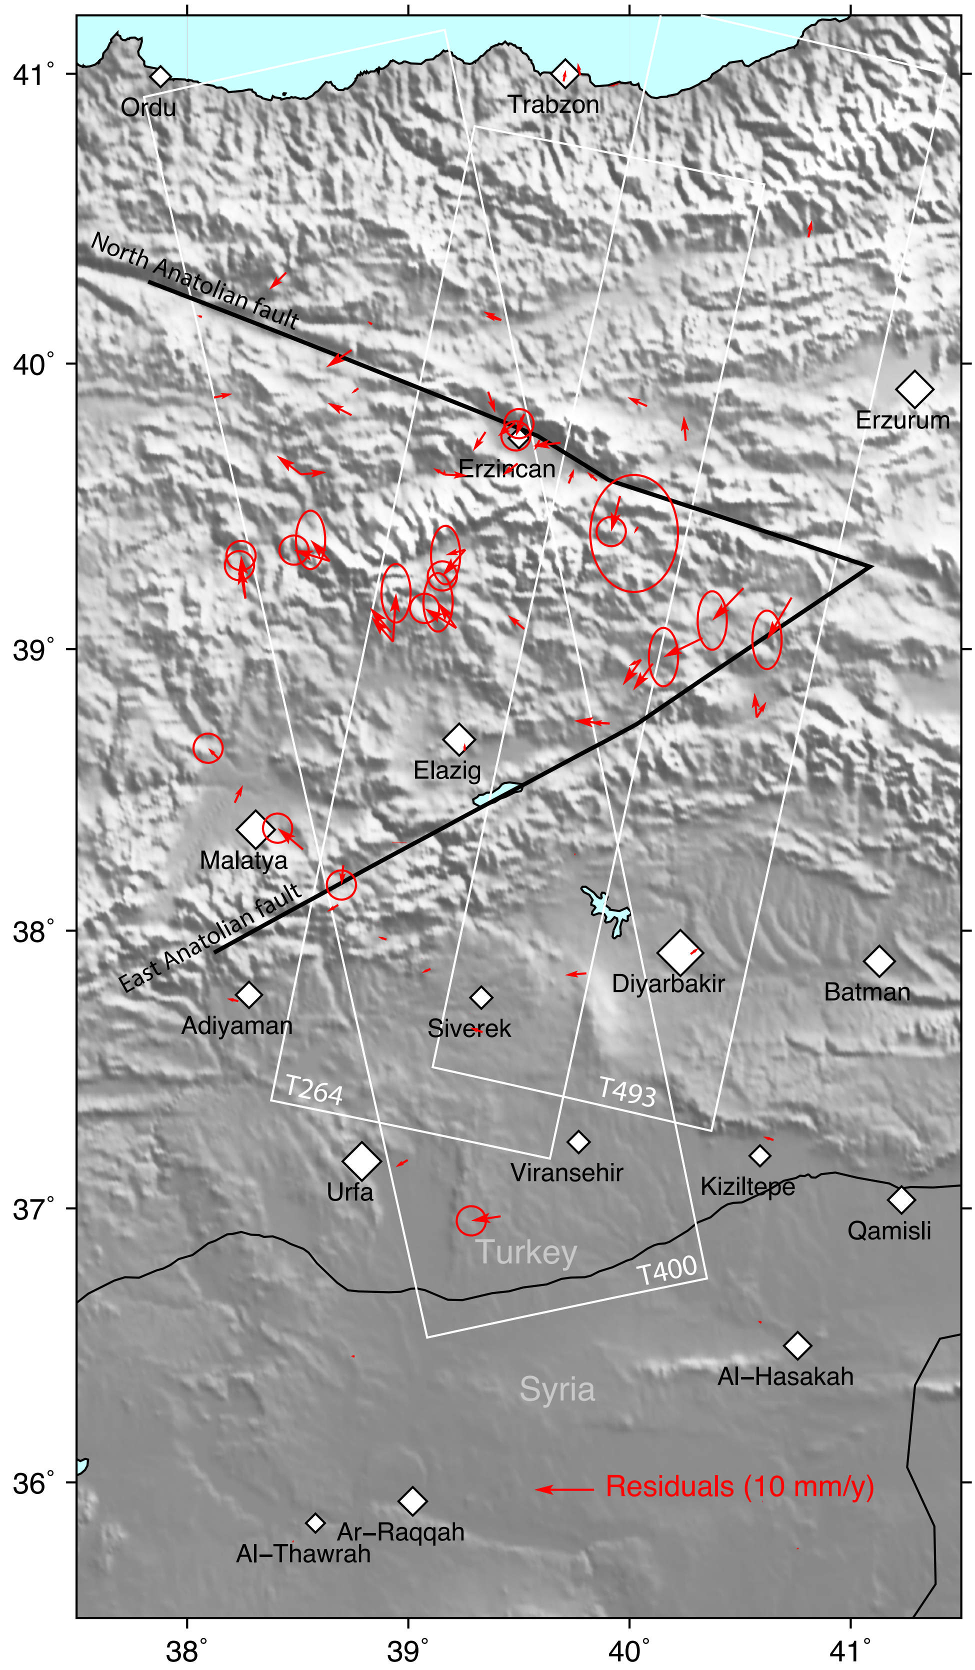


**Figure S13.** GPS Residuals. Ellipses are summed 2-$\sigma$ standard deviations of the observed and predicted data.

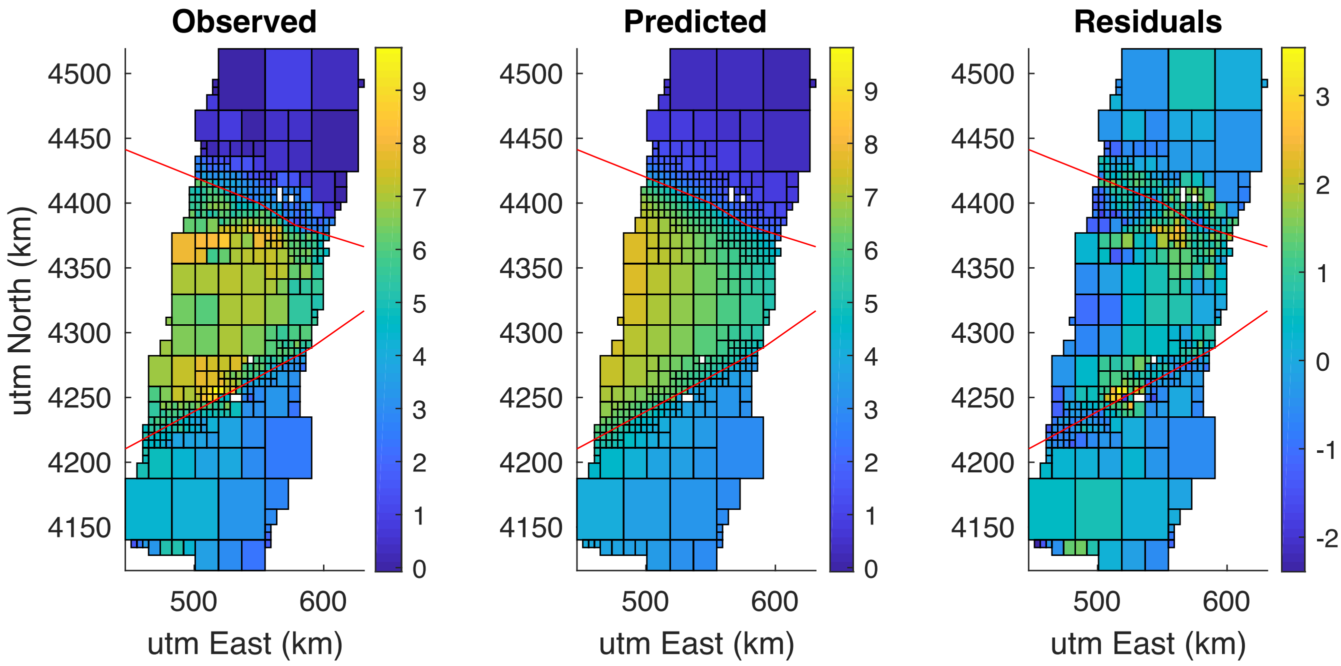


**Figure S14.** Observed (left), predicted (center), and residual (right) sub-sampled SAR interferograms for Track T264. Red lines indicate the fault traces. Units are mm/y in the LOS direction.

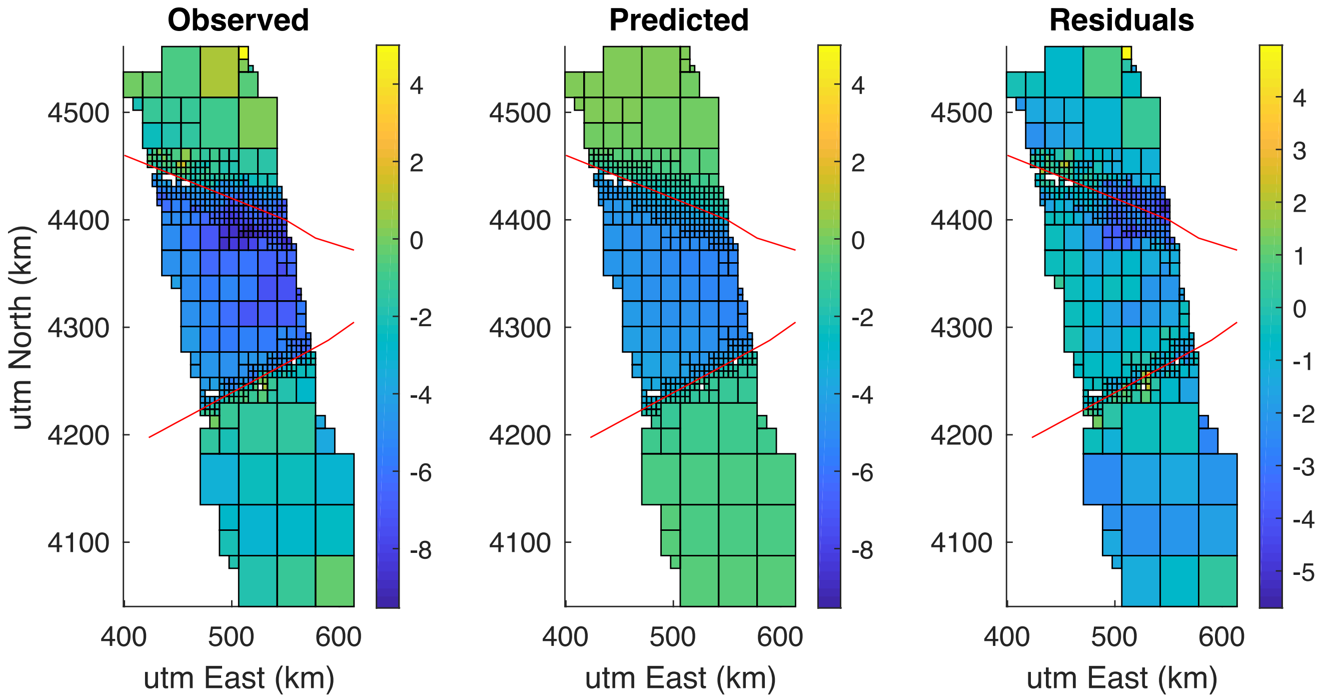


**Figure S15.** Same as Fig. S14 for track T400. Units are mm/y in the LOS direction.

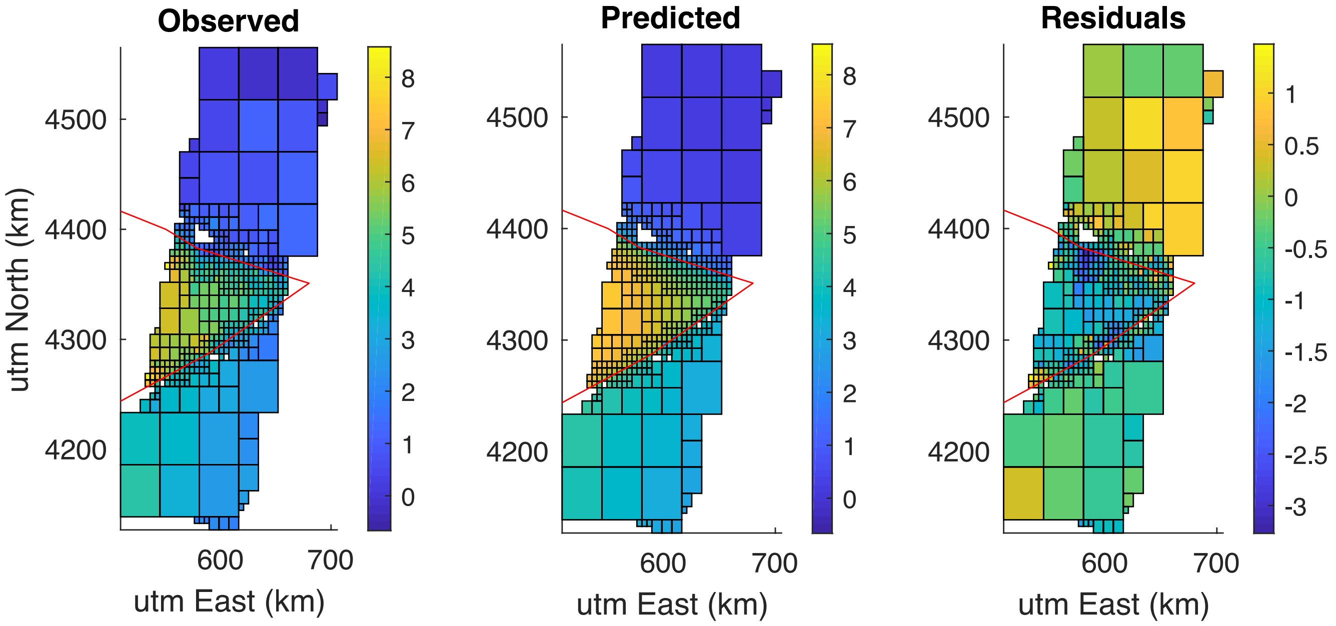


**Figure S16.** Same as Fig. S14 for track T493. Units are mm/y in the LOS direction.

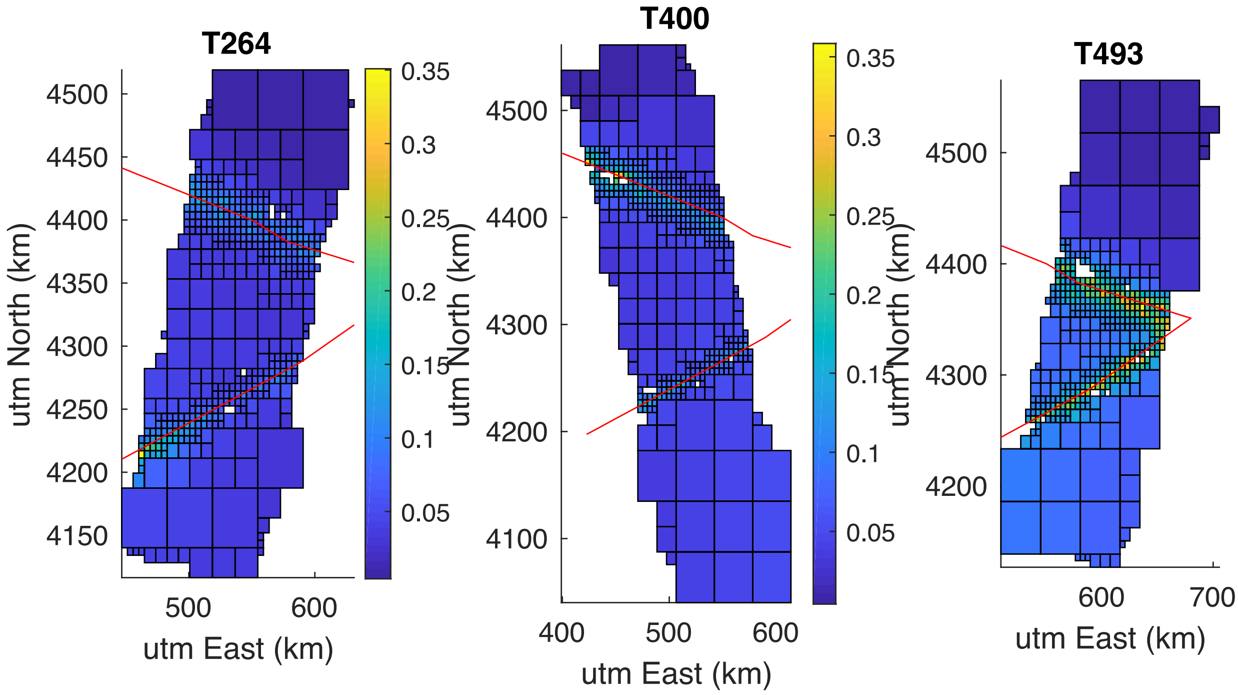


**Figure S17.** Standard deviation of the predicted interferograms. Units are mm/y in the LOS directions.
